# Supplementary material for: LiFUSE: Frequency-Spatial Unified Self-Supervised Pretraining for Liver Disease Analysis on Non-contrast CT
Source: arXiv:2610.18243 source file (2026-10-13)
Supplement: Supplementary file 1 [file appendix.tex]

% \newpage
\appendix
Appendix.
